# Supplementary material for: Magneto-optic Kerr effect in a spin-polarized zero-moment ferrimagnet
Source: arXiv:1806.07719 source file (2018-09-03)
Supplement: Supplementary file 1 [file mnruga-supplement-revised.pdf]

# Supplementary Information:

# Magnetooptical Kerr effect in a zero-moment ferrimagnet: The case of $Mn_2Ru_xGa$

K. Fleischer,[1,2] N. Thiyagarajah,[1,3] Y.-C. Lau,[1,3] D. Betto,[1,3] K. Borisov,[1,3]
C. M. Smith,[1] I. V. Shvets,[1,3] J.M.D. Coey,[1,3] and K. Rode[1,3]

[1]*School of Physics, Trinity College Dublin, Dublin 2, Ireland*
[2]*School of Physical Sciences, Dublin City University, Dublin 9, Ireland*
[3]*CRANN and AMBER, Trinity College Dublin, Dublin 2, Ireland*

## S1. Optical Modeling

As discussed in the manuscript the procedure to extract the individual components ($\tilde{\varepsilon}_{ij}$) of the complex dielectric tensor requires least square fitting of modelled $\tan\Psi$, $\cos\Delta$, $\theta_k$ values over the entire measured spectral range. The standard method to do this for multilayered samples are so called transfer matrix calculations. In ellipsometric measurements of thin films these are typically used to not only derive the dielectric function of a thin film, but can also be used to fit film thickness, surface roughness and other parameter.[1]

The spectral shape of each tensor component is typically described by a set of standard functions, with Drude oscillators, harmonic oscillators (Drude-Lorentz), Tauc-Lorentz or expressions for 1D, 2D, or 3D bulk critical points.[1,2] As the modelling describes the spectral shape of the dielectric functions over the whole spectral range there are often several ways to describe it. Here we have chosen the simplest form, with the least amount of free parameter, in order to investigate systematic changes with Ruthenium concentration. In addition we did not fit on any geometric parameter (film thickness, interface roughness) as these have been independently measured by X-ray reflectance. All other materials (Air, $AlO_x$, MgO) were described by tabulated bulk values of their respective dielectric function. To minimise the number of free parameters all films $Mn_2Ru_xGa$ films have been treated as optical isotropic ($\tilde{\varepsilon}_{xx}=\tilde{\varepsilon}_{yy}=\tilde{\varepsilon}_{zz}$).

In all cases fits began with refining spectra using a single Drude oscillator (two parameters: amplitude $A$ (proportional to plasma frequency) and broadening $\Gamma$ (inverse of scattering rate)). In a second step additional harmonic oscillators (Drude-Lorentz oscillator, three parameter each: amplitude $A$, broadening $\Gamma$, and position $\omega_0$) were added and subsequently refined until any addition of another oscillator did not change the $\chi^2$ value further. This way we ensure that the spectral shape is only described with the minimum number of free fitting parameter. As discussed in the main article for the description of the diagonal component of the dielectric function three such oscillators were required, one in the visible, one in the UV and one in the deep UV range.

Once the diagonal component was refined by the fits to the ellipsometric data for three angles of incidence, the off-diagonal component $\tilde{\varepsilon}_{xy}$ was fitted by calculating the complex Fresnel reflectance $r_x$ of an air/$AlO_x$/$Mn_2Ru_xGa$/MgO stack of known geometry using the refined $\tilde{\varepsilon}_{xx}$, and $r_y$ using $\tilde{\varepsilon}_{xx}+\tilde{\varepsilon}_{xy}$. $\theta_k$ is then simply derived from $\theta_k = Re(r_x - r_y)/(r_x + r_y)$. This equation is valid as we only analyse polar Moke of an optically isotropic medium, measured at near normal incidence. No dependece of the optical spectra on z-components of the dielectric tensor occur, nor difference between $\tilde{\varepsilon}_{xx}$ and $\tilde{\varepsilon}_{yy}$ are expected.[1,3] $\tilde{\varepsilon}_{xy}$ was likewise, initially described by a single Drude oscillator. Additional harmonic oscillators were added to minimise $\chi^2$. As for $\tilde{\varepsilon}_{xx}$ three oscillators were required to describe the spectral shape of $\tilde{\varepsilon}_{xy}$ and accurately describe $\theta_k$. However for $\tilde{\varepsilon}_{xy}$ two individual oscillators in the near infra-red and visible range, yet no DUV contribution were required.

All functions used to describe $\tilde{\varepsilon}_{xx}$ as well as $\tilde{\varepsilon}_{xy}$ are Kramers-Kronig consistent, hence represent meaningful physical fits of the underlying absorption processes, rather than simply reproducing the shape of the spectra. The procedure outlined here, implicitly treats any features in the spectral response of $\theta_k$ caused by variations in stack reflectance caused by the spectral shape of the dielectric function of all materials involved, as well as thickness related thin film interference structures.

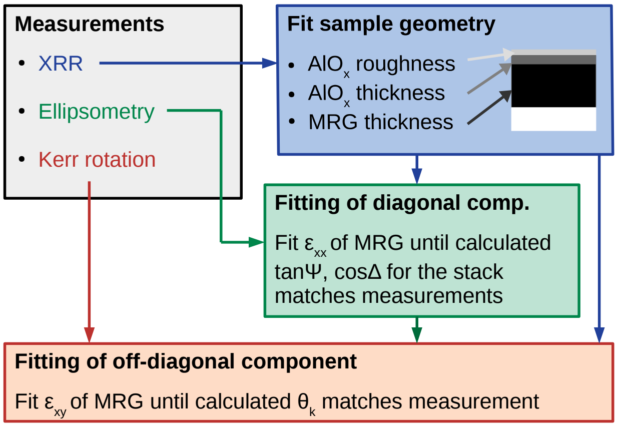


**Supplementary Figure S1.**
Schematic of the information flow for the optical modeling used to derive the tensor components for the dielectric tensor of $Mn_2Ru_xGa$. The procedure is done for each sample, to compare $\tilde{\varepsilon}_{xx}$, and $\tilde{\varepsilon}_{xy}$ as function of Ruthenium content.

## S2. Deconvolution of contributions to the dielectric tensor – dependence on Ru concentration

### 1. *Diagonal component* $\varepsilon_{xx}, \sigma_{xx}$

In the main article (Fig. 4) we show the dielectric function $\tilde{\varepsilon}_{xx}$ for several samples as extracted from least square fits of the measured $\tan\Psi$ and $\cos\Delta$. The deconvolution into several components, as shown in the article (Fig. 5)

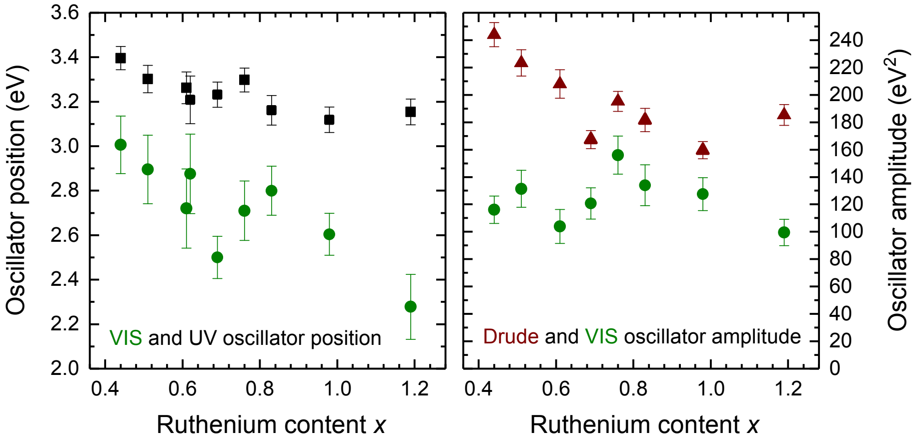


**Supplementary Figure S2.** Dependence of selected parameter of the model dielectric tensor as function of the Ru content. Here we show parameter with a significant change upon increase of Ru content such as the energetic positions for the VIS and UV oscillator and the amplitude of the Drude and VIS oscillators.

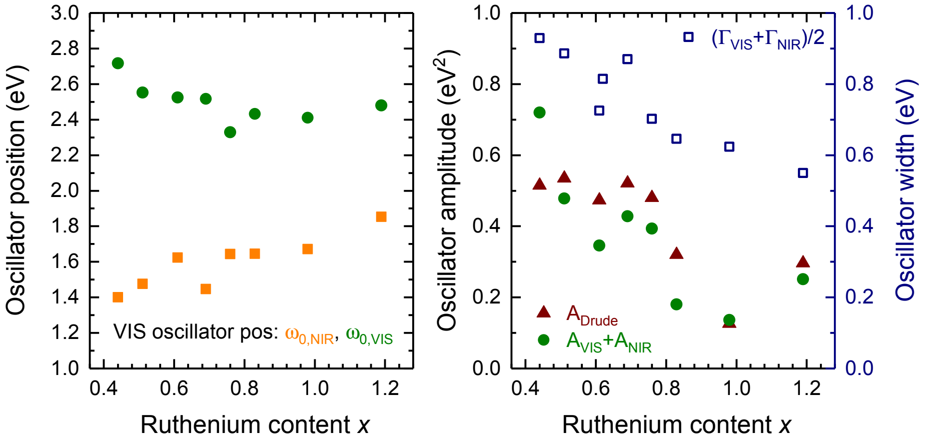


**Supplementary Figure S3.** Spectral position of the two interband components used to describe $\tilde{\varepsilon}_{xy}$. Amplitude of the fitted interband and intra-band (Drude) components of $\tilde{\varepsilon}_{xy}$, as well as their average oscillator width ($\Gamma$). The energetic positions and line widths, again consistently change with the Ru content.

for a sample with $x = 0.61$, was likewise done for all investigated samples. We can therefore analyse the dependence of individual components on the Ru content.

Figure S1 shows selected parameters extracted from the dielectric model as function of Ru content. Both the Drude part as well as the main, VIS Oscillator are very broad, with a broadening parameter of the harmonic oscillator ($\Gamma \approx 5$-$7\,eV$) larger than the measured range. As discussed, this is due to each model oscillator being a superposition of a larger number of unresolved optical transitions. An increase in Ru concentration leads to an apparent red shift of absorption structures, in particular for the VIS component, which we assign to Mn states. We have shown[4] that on increasing $x$, the bands originating from Mn in the 4$c$ position (higher-energy final states) is preferentially filled by the added electrons. Consequently this reduces the number of unoccupied states, skewing the relative weights of the different oscillators contributing to the broad VIS absorption, leading to the red-shift in energy. The Drude component is also affected by the Ru content. The DC conductivity of $Mn_2Ru_xGa$ varies by approximately 30 %[5] when $x$ is changed from 0.6 to 1.0, consistent with our observation of altered amplitudes in the Drude tail.

The presence of two dominant interband absorption structures, as well as the amplitude of the inter-band transitions is very similar to previous reports on cubic $Ni_2MnGa$.[6] Noticeably the two distinct absorption structures are less well separated and much broader in $Mn_2Ru_xGa$ than for $Ni_2MnGa$, again due to Mn occupying two different crystallographic positions.

Broadening of optical transitions is generally associated with disorder and has been seen for $Ni_2MnGa$[6], as well as $Co_2CrAl$.[7] In our case the observed differences with increasing Ru content, are significantly smaller than those reported for e.g. amorphous to crystalline samples of $Co_2CrAl$.[7] In addition the peak widths of inter-band transitions are slightly decreasing with inclusion of Ru, consistent with a better atomic order, once the initially vacant 4d-sites are occupied. Crystalline long-range quality, determined by XRD, is similar for all samples, and we conclude that the variations with $x$ are dominated by changes of the local order and Mn band filling, rather than disorder.

### 2. *Off-diagonal component* $\varepsilon_{xy}, \sigma_{xy}$

Similarly the Kerr spectra show features in the IR, associated to the intra-band transitions (Drude-like tail). In contrast to $\tilde{\varepsilon}_{xx}$ the magnetic components $\tilde{\varepsilon}_{xy}$ are dominated by the two inequivalent Mn sites and more fine structure is resolvable. We therefore need two individual components to describe the broad VIS oscillator in the Kerr-spectra. These are assigned two involve the Mn-4$a$ and Mn-4$c$ respectively. Our previous XAS/MCD measurements[4] showed that the magnetic moment in $Mn_2Ru_xGa$ is entirely carried by Mn. To compare the spectral dependence of the off-diagonal component of the dielectric tensor

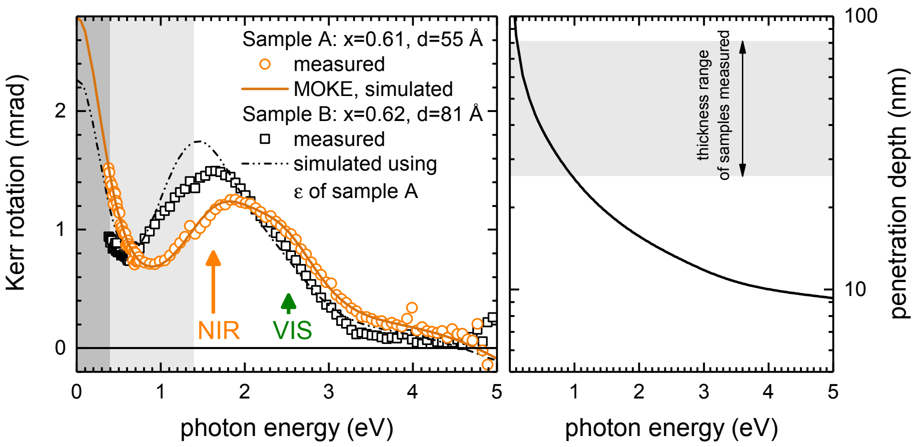


**Supplementary Figure S4.** Measured MOKE spectra of two samples with comparable $x$ but grown at different growth rates. The optical model of the thinner sample is used to calculate the expected MOKE of the thicker, highlighting the thickness dependence of the raw MOKE signal and the real change in magnetic order between the two samples. The right panel shows the penetration depth of light in $Mn_2Ru_xGa$ calculated from $\tilde{\varepsilon}_{xx}$ of a sample with $x = 0.61$. Please note the logarithmic scale.

$\tilde{\varepsilon}_{xy} = \pm iQm_z\tilde{\varepsilon}_{xx}$ between samples we only consider the magnitude of the Kerr rotation and only analyse fully saturated samples. After modelling the $\theta_k$ spectra using individual components in $\tilde{\varepsilon}_{xy}$, it is noticeable that all parameters show monotonic changes with $x$ (see Fig. S3). Particular the two features associated with interband transitions in the NIR-VIS (Mn) region show shifts in energetic position and amplitude, with distinctly different rate of change before and after $x \approx 0.7$. The latter has also been observed in the change of Mn 4$c$ magnetisation as function of $x$,[4] again suggesting that these particular optical transitions involve electronic states localised at the Mn sites. Likewise the fitted broadening of the structures is reduced with increasing Ru content as the number of crystal vacancies is reduced when $x$ approaches 1, and the local order is increased.

### S3. Thickness dependence in MOKE

For thin films there is no simple analytical equation to correlate the Kerr rotation $\theta_k$ to $\tilde{\varepsilon}_{xy}$. The film thickness for layers analysed here, varies between 26 and 81 nm. This coverage regime can not be treated either as thin film, nor optical thick layer as the layer thickness is not significantly larger than the penetration depth of light (see Fig. S4). Hence full optical transfer matrix calculations are required to fit the spectral form of $\tilde{\varepsilon}_{xy}$ to the measured $\theta_k$ spectra.[8] The main article Fig. 4 shows the raw MOKE measurements and Fig. 5 and 6 the model off-diagonal tensor components of the dielectric function (as fitted MOKE and in terms of $\sigma$).

The full optical modeling of the dielectric tensor components can now also be used to illustrate the dependency of measured $\theta_k$ spectra on the thickness of a thin film. Even with no changes in a materials electronic and magnetic properties, the spectral form and magnitude of the $\theta_k$ signal will strongly depend on the thickness of the thin film, as long as the light penetration depth is larger or in the same order as the film thickness. Figure S4 illustrates the expected Kerr rotation for varying film thickness. We show two nominally identical samples with different thickness, and then use the fit of the thinner sample to model the thicker. We find a very good agreement between the model and spectral features of the thicker sample, but difference in amplitude are observed. This illustrates the deviations in magnetic ordering between samples of different thickness as previously reported.[9] Independent from our discussion specific to $Mn_2Ru_xGa$ this illustrates the importance of employing optical models to quantitatively discuss sample properties in magnetic thin films, rather than discussing raw MOKE data.


[1] G. E. Jellison, in *Handbook of Ellipsometry*, edited by H. G. Tompkins and E. A. Irene (William Andrew Publishing, Norwich, NY, 2005) pp. 237 – 296.

[2] P. Y. Yu and M. Cardona, *Fundamentals of semiconductors* (Springer, 2005).

[3] T. Herrmann, K. Lüdge, W. Richter, K. G. Georgarakis, P. Poulopoulos, R. Nünthel, J. Lindner, M. Wahl, and N. Esser, Phys. Rev. B **73**, 134408 (2006).

[4] D. Betto, N. Thiyagarajah, Y.-C. Lau, C. Piamonteze, M.-A. Arrio, P. Stamenov, J. Coey, and K. Rode, Phys. Rev. B **91**, 094410 (2015).

[5] N. Thiyagarajah, Y.-C. Lau, D. Betto, K. Borisov, J. Coey, P. Stamenov, and K. Rode, Appl. Phys. Lett. **106**, 122402 (2015).

[6] Y. V. Kudryavtsev, Y. Lee, and J. Rhee, Phys. Rev. B **66**, 115114 (2002).

[7] Y. Kudryavtsev, V. Uvarov, V. Oksenenko, Y. Lee, J. Kim, Y. Hyun, K. Kim, J. Rhee, and J. Dubowik, Phys. Rev. B **77**, 195104 (2008).

[8] J. Zak, E. Moog, C. Liu, and S. Bader, Phys. Rev. B **43**, 6423 (1991).

[9] M. Žic, K. Rode, N. Thiyagarajah, Y.-C. Lau, D. Betto, J. M. D. Coey, S. Sanvito, K. J. O'Shea, C. A. Ferguson, D. A. MacLaren, and T. Archer, Phys. Rev. B **93**, 140202 (2016).
